# Supplementary material for: SciHorizon-DataEVA: An Agentic System for AI-Readiness Evaluation of Heterogeneous Scientific Data
Source: arXiv:2604.26645 source file (2026-05-28)
Supplement: Supplementary file 1 [file elements_define.tex]

\begin{table*}[h]
\centering
\caption{Evaluation framework (Part I): Governance Trustworthiness (FAIRness, provenance \& licensing, and scientific ethics).}
\label{tab:evaluation_framework_gov}
\begin{tabular}{p{0.12\textwidth} p{0.18\textwidth} p{0.20\textwidth} p{0.44\textwidth}}
\toprule
\textbf{Dimension} & \textbf{Sub-dimension} & \textbf{Element} & \textbf{Detailed Definition} \\
\midrule
\multirow{10}{*}{\textbf{Gov. Trust.}} 
    & \multirow{4}{=}{\textbf{FAIRness Principles}} 
        & Metadata Findability 
        & Presence of persistent identifiers (e.g., DOI, Handles) and indexed metadata to ensure the dataset can be located by humans and machines. \\
    &   & Access Transparency 
        & Clarity of the access protocols, including authentication requirements and data retrieval methods. \\
    &   & Interoperability 
        & Use of formal, accessible, and shared languages for knowledge representation (e.g., RDF, JSON-LD) and standard vocabularies. \\
    &   & Reusability Metadata 
        & Availability of rich documentation, including usage scopes and domain-specific attributes that facilitate accurate reuse. \\
    \cmidrule{2-4}
    & \multirow{3}{=}{\textbf{Provenance \& Licensing}} 
        & Licensing Clarity 
        & Explicit specification of legal terms (e.g., Creative Commons, MIT) defining redistribution and modification rights. \\
    &   & Attribution Rights 
        & Clearly defined ownership and required citation formats to ensure intellectual property is respected. \\
    \cmidrule{2-4}
    & \multirow{3}{=}{\textbf{Scientific Ethics}} 
        & Consent Compliance 
        & Verifiable evidence that data collection involving human subjects or sensitive ecosystems adheres to institutional informed consent. \\
    &   & Dual-Use Risk 
        & Assessment of whether the data poses security risks (e.g., biological or nuclear) if used for purposes other than intended research. \\
    &   & Privacy Protection 
        & Verification of de-identification and anonymization rigor to prevent the leakage of sensitive or personally identifiable information. \\
\bottomrule
\end{tabular}
\end{table*}

% =================== Part II: Data Quality ===================
\begin{table*}[h]
\centering
\caption{Evaluation framework (Part II): Data Quality (completeness, consistency, accuracy, and uniqueness).}
\label{tab:evaluation_framework_quality}
\begin{tabular}{p{0.12\textwidth} p{0.18\textwidth} p{0.20\textwidth} p{0.44\textwidth}}
\toprule
\textbf{Dimension} & \textbf{Sub-dimension} & \textbf{Element} & \textbf{Detailed Definition} \\
\midrule
\multirow{10}{*}{\textbf{Data Qual.}} 
    & \multirow{3}{=}{\textbf{Completeness}} 
        & Asset Integrity 
        & Detects corruption, zero-byte files, or decoding failures in unstructured data (images, audio, sequences) to ensure readability. \\
    &   & Table Null Rate 
        & Calculates the ratio of missing values (NaN, None, NULL) in structured tables or metadata fields. \\
    &   & Modal Alignment 
        & Checks for linkage breaks in multi-modal datasets (e.g., images missing labels, or references missing source tables). \\
    \cmidrule{2-4}
    & \multirow{2}{=}{\textbf{Consistency}} 
        & Tensor Shape Consistency 
        & Verifies uniformity in dimension and shape across samples (e.g., all images are $224{\times}224{\times}3$) to enable batch training. \\
    &   & Type Consistency 
        & Checks for data type purity within columns of weak-typed formats (e.g., CSV/JSON) to prevent parsing errors. \\
    \cmidrule{2-4}
    & \multirow{3}{=}{\textbf{Accuracy}} 
        & Label Noise Detection 
        & Uses algorithms like Confident Learning to identify potentially mislabeled samples in supervised datasets. \\
    &   & Measurement Sanity 
        & Detects anomalies such as stuck values, non-physical negatives (e.g., mass), or underutilized bit-depth in sensor data. \\
    &   & Schema Validity 
        & Evaluates if specific entities (e.g., SMILES, DNA sequences) comply with their defined regex patterns or encoding standards. \\
    \cmidrule{2-4}
    & \textbf{Uniqueness} 
        & Duplication Check 
        & Identifies exact duplicate records or primary key (ID) collisions that occur during data entry or processing. \\
\bottomrule
\end{tabular}
\end{table*}

% =================== Part III: AI Compatibility ===================

\begin{table*}[h]
\centering
\caption{Evaluation framework (Part III): AI Compatibility (model adaptability, scale, balance, feature utility, and data point value).}
\label{tab:evaluation_framework_ai}
\begin{tabular}{p{0.12\textwidth} p{0.18\textwidth} p{0.20\textwidth} p{0.44\textwidth}}
\toprule
\textbf{Dimension} & \textbf{Sub-dimension} & \textbf{Element} & \textbf{Detailed Definition} \\
\midrule
\multirow{11}{*}{\textbf{AI Comp.}} 
    & \multirow{2}{=}{\textbf{AI Model Adaptability}} 
        & Geometric Architecture Fit 
        & Recommends foundational model architectures (CNN, GNN, Transformer) based on data topology (Grid, Graph, Sequence). \\
    &   & Task \& Strategy Fit 
        & Recommends advanced strategies (Diffusion, Offline RL) based on task objectives and data scale. \\
    \cmidrule{2-4}
    & \multirow{2}{=}{\textbf{Data Scale}} 
        & Domain Scale Tier 
        & Classifies sample size (Few-shot/Mid/Large) based on domain-specific thresholds rather than absolute counts. \\
    &   & N/D Ratio 
        & Evaluates the ratio of sample size ($N$) to effective feature dimension ($D$) to assess potential overfitting risks. \\
    \cmidrule{2-4}
    & \multirow{2}{=}{\textbf{Class Balance}} 
        & Target Distribution Health 
        & Measures label distribution using entropy (classification) or skewness and kurtosis (regression). \\
    &   & Minority Support 
        & Checks if the absolute number of samples in the minority class meets the minimum requirements for stable learning. \\
    \cmidrule{2-4}
    & \multirow{2}{=}{\textbf{Feature Importance}} 
        & Statistical Mutual Info 
        & Calculates the correlation strength (linear/non-linear) between the feature matrix $X$ and target $Y$. \\
    &   & Feature Redundancy 
        & Identifies collinearity and intrinsic dimensionality of the feature set to reduce computational waste. \\
    \cmidrule{2-4}
    & \textbf{Data Point Value} 
        & Data Shapley Value 
        & Quantifies the marginal contribution of individual samples to model performance using KNN-Shapley approximations. \\
\bottomrule
\end{tabular}
\end{table*}

% =================== Part IV: Scientific Adaptability ===================

\begin{table*}[h]
\centering
\caption{Evaluation framework (Part IV): Scientific Adaptability (generalizability, scarcity, causal completeness, and condition coverage).}
\label{tab:evaluation_framework_sci}
\begin{tabular}{p{0.12\textwidth} p{0.18\textwidth} p{0.20\textwidth} p{0.44\textwidth}}
\toprule
\textbf{Dimension} & \textbf{Sub-dimension} & \textbf{Element} & \textbf{Detailed Definition} \\
\midrule
\multirow{14}{*}{\textbf{Sci. Adapt.}} 
    & \multirow{2}{=}{\textbf{Task Generalizability}} 
        & Task Archetype Support 
        & Evaluates if column combinations support four major tasks: Prediction, Inverse Generation, Dynamics, and Discovery. \\
    &   & Semantic Concept Span 
        & Measures the breadth of scientific topics covered by mapping metadata to top-level ontology branches. \\
    \cmidrule{2-4}
    & \multirow{3}{=}{\textbf{Data Scarcity}} 
        & Source Complexity 
        & Assesses hardware/environmental barriers involved in data generation (Simulation vs. Lab vs. Extreme Observation). \\
    &   & Spatiotemporal Uniqueness 
        & Checks if data captures non-repeatable historical events or transient phenomena (e.g., supernovae, pandemics). \\
    &   & Annotation Dependency 
        & Evaluates the cognitive barrier required to label the data (Crowdsourcing vs. Domain Experts). \\
    \cmidrule{2-4}
    & \multirow{3}{=}{\textbf{Causal Completeness}} 
        & Interventionality 
        & Distinguishes between active intervention (RCT/Experiment) and passive observation for causal inference. \\
    &   & Process Resolution 
        & Checks for the presence of evolutionary paths or dynamic processes rather than just terminal states. \\
    &   & Environmental Completeness 
        & Verifies if critical context parameters (e.g., temperature, instrument settings) are recorded to prevent confounding. \\
    \cmidrule{2-4}
    & \multirow{3}{=}{\textbf{Condition Coverage}} 
        & Parameter Space Span 
        & Ratio of the covered physical parameter range relative to theoretical or engineering boundaries. \\
    &   & Regime/Phase Diversity 
        & Checks if the data distribution crosses critical phase transition points or exhibits multi-modal behavior. \\
    &   & Boundary Exploration 
        & Evaluates the proportion of samples representing extreme conditions or failure/negative cases. \\
\bottomrule
\end{tabular}
\end{table*}
