# Supplementary material for: SciHorizon-DataEVA: An Agentic System for AI-Readiness Evaluation of Heterogeneous Scientific Data
Source: arXiv:2604.26645 source file (2026-05-28)
Supplement: Supplementary file 2 [file evidence_bp.tex]

% \begin{table*}[t]
% \centering
% \caption{\textcolor{red}{Evidence table of datasets, dimensions, scores, and supporting quotations.}}
% \label{tab:evidence_dataset}

% \setlength{\tabcolsep}{4pt}
% \renewcommand{\arraystretch}{1.18}

% \resizebox{\textwidth}{!}{%
% \begin{tabular}{p{5.4cm}|p{4.6cm} c p{4.2cm} p{9.8cm}}
% \toprule
% \textbf{Dataset} & \textbf{Dimension} & \textbf{Score} & \textbf{Article} & \textbf{Evidence} \\
% \midrule

% \texttt{Ionospheric\_Observations} &
% Scientific Adaptability &
% 97 &
% Mechanism for Sporadic E enhancement during the May 2024 geomagnetic storm: TIEGCM simulation, \textit{Journal of Geophysical Research: Space Physics}, 2025 &
% ``Geomagnetic storms can inject a large amount of energy into the polar regions. This energy then propagates to lower latitudes, resulting in extreme changes in the thermospheric composition, ionospheric plasma density (e.g., Fu et al., 2025; \dots\ Yang et al., \dots) as well as the neutral atmospheric circulation.'' \\
% \midrule

% \multirow{2}{*}{\texttt{Circular\_Polarization}} &
% \multirow{2}{=}{Scientific Adaptability (Data Scarcity)} &
% 98 &
% Linear to circular conversion in the polarized radio emission of a magnetar, \textit{Nature Astronomy}, 2024 &
% ``The RM evolutions of these objects are probably the result of slow changes in the particle density and magnetic fields of their local environments. More recently, large RM variations and significant levels of circular polarization have been detected in at least three other repeating FRB sources [56--58].'' \\
% \cmidrule(l){2-5}
% & & 87 &
% A persistently active fast radio burst source embedded in an expanding supernova remnant, \textit{Science Bulletin}, 2025 &
% ``The complexity of its environment is also reflected in the detection of rare circular polarization and a highly stochastic, Brownian motion--like bursting behavior in the time--energy domain [7, 8].'' \\
% \midrule

% \texttt{Galileo\_observation} &
% Scientific Adaptability (Data Scarcity) &
% 87 &
% A slot region in the magnetosphere of Jupiter, \textit{Nature Communications}, 2025 &
% ``Multiple dawn--dusk asymmetries have been reported within Jupiter's magnetosphere, especially the corresponding charged particle distributions [37--41].'' \\
% \bottomrule
% \end{tabular}%
% }
% \end{table*}

% \begin{table*}[t]
% \centering
% \caption{\textcolor{red}{Evidence table of datasets, dimensions, scores, and supporting quotations.}}
% \label{tab:evidence_dataset}

% \setlength{\tabcolsep}{4pt}
% \renewcommand{\arraystretch}{1.18}

% \resizebox{\textwidth}{!}{%
% \begin{tabular}{p{3.0cm}|p{3.6cm} c p{5.0cm} p{12.4cm}}
% \toprule
% \textbf{Dataset} & \textbf{Dimension} & \textbf{Score} & \textbf{Article} & \textbf{Evidence} \\
% \midrule

% \multirow{2}{*}{\texttt{Circular\_Polarization}} &
% Data Scarcity &
% 100.0 &
% Linear to circular conversion in the polarized radio emission of a magnetar, \textit{Nature Astronomy}, 2024 &
% ``The RM evolutions of these objects are probably the result of slow changes in the particle density and magnetic fields of their local environments. More recently, large RM variations and significant levels of circular polarization have been detected in at least three other repeating FRB sources.'' \\
% \cmidrule(l){2-5}
% &Data Scarcity & 100.0 &
% A persistently active fast radio burst source embedded in an expanding supernova remnant, \textit{Science Bulletin}, 2025 &
% ``The complexity of its environment is also reflected in the detection of rare circular polarization and a highly stochastic, Brownian motion--like bursting behavior in the time--energy domain.'' \\
% \midrule

% \texttt{Galileo\_observation} &
% Data Scarcity &
% 100.0 &
% A slot region in the magnetosphere of Jupiter, \textit{Nature Communications}, 2025 &
% ``Multiple dawn--dusk asymmetries have been reported within Jupiter's magnetosphere, especially the corresponding charged particle distributions.'' \\
% \midrule

% % -------------------- Added block: TAA (3 rows) --------------------
% \multirow{2}{*}{\texttt{TAA}} &
% Task Generalizability &
% 90.0 &
% \multirow{2}{=}{Database of ternary amorphous alloys based on machine learning, \textit{Chinese Physics B}, 2025} &

%  ``Other alloy systems can also be predicted using the same workflow.'' \\
% \cmidrule(l){2-3}\cmidrule(l){5-5}

% & Data Scale &
% 100.0 &
% & ``This indicates that our database encompasses a broad range of elements known to form amorphous alloys.'' \\
% % ------------------ End of added block: TAA ------------------


% \midrule


% \multirow{2}{*}{\texttt{BigSolDBv2}} &
% Class Balance &
% 80.1 &
% \multirow{2}{=}{BigSolDB 2.0, dataset of solubility values for organic compounds in different solvents at various temperatures, \textit{Scientific Data}, 2025} &

%  ``In this study, we present a dataset containing 103944 experimental solubility values within a temperature range from 243 to 425 K for 1448 organic compounds measured in 213 individual solvents extracted from 1595 peer-reviewed articles. '' \\
% \cmidrule(l){2-3}\cmidrule(l){5-5}

% & AI Model Adaptability &
% 89.2 &
% & ``Moreover, this dataset paves the way to train machine learning models for solubility prediction in a wide variety of organic solvents which can be extremely useful in the design of many chemical and technological processes.'' \\


% \midrule


% \multirow{2}{*}{\texttt{FreeSolv}} &
% Completeness &
% 100.0 &
% \multirow{2}{=}{BigSolDB 2.0, dataset of solubility values for organic compounds in different solvents at various temperatures, \textit{Scientific Data}, 2025} &

%  ``The starting point in constructing the FreeSolv database was to pull together all of the lead author’s previous work calculating hydration free energies in explicit solvent. This included calculated values, experimental values, and structures and input files2 from several previous studies.'' \\
% \cmidrule(l){2-3}\cmidrule(l){5-5}

% & Accuracy &
% 100.0 &
% & ``we had retained not only calculated and experimental hydration free energies and original coordinate files (.mol2 format) containing geometries and partial charges, but also input files in the form of GROMACS topology and coordinate files.'' \\

% \midrule

% \multirow{3}{*}{\texttt{EuroSAT}} &
% Class Balance &
% 99.8 &
% \multirow{2}{=}{EuroSAT: A Novel Dataset and Deep Learning Benchmark for Land Use and Land Cover Classification，\textit{IEEE Journal of Selected Topics in Applied Earth Observations and Remote Sensing}, 2019} &
% ``We present a novel dataset, based on these images that covers 13 spectral bands and is comprised of ten classes with a total of 27 000 labeled and geo-referenced images.'' \\
% \cmidrule(l){2-3}\cmidrule(l){5-5}

% & Task Generalizability &
% 81.6 &
% & ``The resulting classification system opens a gate toward a number of earth observation applications. We demonstrate how this classification system can be used for detecting land use and land cover changes, and how it can assist in improving geographical maps.'' \\

% \cmidrule(l){2-5}

% & AI Model Adaptability &
% 88.9 &
% Toward Explainable AI in Satellite Imagery: A ResNet-50-Based Study on EuroSAT Classification, \textit{IEEE Access}, 2025 &
% ``Leveraging a pre-trained ResNet-50 model on the EuroSAT dataset, we analyzed twenty representative satellite image samples, comprising both correctly and incorrectly classified instances across ten land use classes.'' \\


% \midrule

% \multirow{5}{*}{\texttt{MedMNISTv2}} &
% Completeness &
% 100.0 &
% \multirow{4}{=}{MedMNIST v2 - A large-scale lightweight benchmark for 2D and 3D biomedical image classification, \textit{Scientific Data}, 2023} &
% ``we provide an official train-validation-test split for each subset. We use the official data split from source dataset (if provided) to avoid data leakage'' \\
% \cmidrule(l){2-3}\cmidrule(l){5-5}
% & Accuracy &
% 100.0 & &
% ``Three neuroscience experts segment a pyramidal neuron within the whole volume and proofread all the synapses'' \\
% \cmidrule(l){2-3}\cmidrule(l){5-5}
% & AI Model Adaptability &
% 70.0 & &
% ``For MedMNIST2D, we first implement ResNets10 with a simple early-stopping strategy on validation set as baseline methods'' \\
% \cmidrule(l){2-3}\cmidrule(l){5-5}
% & Task Generalizability &
% 85.0 & &
% ``MedMNIST has been particularly useful for machine learning and computer vision research, e.g., AutoML, trustworthy machine learning'' \\
% \cmidrule(l){2-5}
% & Class Balance &
% 80.3 &
% MedMNIST v2 - A large-scale lightweight benchmark for 2D and 3D biomedical image classification, \textit{Scientific Data}, 2023 &
% ``All images are pre-processed into a MNIST-like format, i.e., 28 × 28 (2D) or 28 × 28 × 28 (3D), with cubic spline interpolation'' \\
% \midrule

% \texttt{FIVES} &
% Task Generalizability &
% 87.5 &
% FIVES: A Fundus Image Dataset for Artificial Intelligence based Vessel Segmentation, \textit{Scientific Data}, 2022 &
% ``Retinal vasculature is a reliable reflection of vessel morphologic changes, which have been demonstrated to relate to numerous clinical conditions'' \\
% \midrule

% \multirow{2}{*}{\texttt{ticks\_in\_China}} &
% Accuracy &
% 81.9 &
% \multirow{2}{=}{A dataset of distribution and diversity of ticks in China, \textit{Scientific Data}, 2019} &
% ``After the data were entered, a second person checked the dataset thoroughly to avoid errors and duplications'' \\
% \cmidrule(l){2-3}\cmidrule(l){5-5}
% & Task Generalizability &
% 100.0 & &
% ``The dataset described here can be used to investigate the spatio-temporal dynamics of tick distribution at multiple scales'' \\
% \midrule

% \multirow{3}{*}{\texttt{miRTarBase\_MTI}} &
% Accuracy &
% 99.5 &
% \multirow{2}{=}{miRTarBase update 2022: an informative resource for experimentally validated miRNA–target interactions, \textit{Nucleic Acids Research}, 2022} &
% ``The database has accumulated >2 200 449 verified MTIs from 13 389 manually curated articles and CLIP-seq data.'' \\
% \cmidrule(l){2-3}\cmidrule(l){5-5}
% & Task Generalizability &
% 65.4 & &
% ``miRTarBase can be applied to miRNA-related disease treatment and drug development.'' \\
% \cmidrule(l){2-5}
% & AI Model Adaptability &
% 95.0 &
% Significant improvement of miRNA target prediction accuracy in large datasets using meta-strategy based on comprehensive voting and artificial neural networks, \textit{BMC Genomics}, 2020 &
% ``The final model of MirTarDANN actually contains eleven modules, including one DANN-4, four DANN-3x, and six DANN-2x modules. Each of the modules is trained and validated in its corresponding subset'' \\
% \midrule

% \multirow{3}{*}{\texttt{SUSTech-SYSU}} &
% Accuracy &
% 70.2 &
% \multirow{3}{=}{The SUSTech-SYSU dataset for automatically segmenting and classifying corneal ulcers, \textit{Scientific Data}, 2020} &
% ``The quality of all the 712 fluorescein staining images used in this study has been visually examined by experienced ophthalmologists to ensure sufficient image quality'' \\
% \cmidrule(l){2-3}\cmidrule(l){5-5}
% & AI Model Adaptability &
% 89.7 & &
% ``this dataset is not only useful for developing and evaluating automated corneal ulcer segmentation algorithms but also beneficial for inventing and validating classification algorithms for identifying the general and specific ulcer patterns as well as the ulcer severity degree'' \\
% \cmidrule(l){2-3}\cmidrule(l){5-5}
% & Task Generalizability &
% 89.3 & &
% ``useful for developing and evaluating automated corneal ulcer segmentation algorithms but also beneficial for inventing and validating classification algorithms'' \\
% \midrule

% \multirow{3}{*}{\texttt{COMPAS\_Analysis}} &
% Completeness &
% 98.7 &
% \multirow{3}{=}{The accuracy, fairness, and limits of predicting recidivism, \textit{Science Advances}, 2018} &
% ``This database of 7214 defendants contains individual demographic information, criminal history, the COMPAS recidivism risk score.'' \\
% \cmidrule(l){2-3}\cmidrule(l){5-5}
% & AI Model Adaptability &
% 95.1 & &
% ``despite COMPAS's collection of 137 features, the same accuracy can be achieved with a simple linear classifier with only two features'' \\
% \cmidrule(l){2-3}\cmidrule(l){5-5}
% & Task Generalizability &
% 100.0 & &
% ``Data-driven, decision-making technologies used in the justice system to inform decisions about bail, parole, and prison sentencing are biased against historically marginalized groups'' \\
% \midrule

% \multirow{3}{*}{\texttt{HIGGS}} &
% Completeness &
% 100.0 &
% \multirow{2}{=}{Searching for exotic particles in high-energy physics with deep learning, \textit{Nature Communications}, 2014} &
% ``The data was produced using Monte Carlo simulations of physics events. It contains 21 kinematic properties measured by the particle detectors in the accelerator. It also contains seven additional derived physics quantities of the particles.'' \\
% \cmidrule(l){2-3}\cmidrule(l){5-5}
% & AI Model Adaptability &
% 100.0 & &
% ``Figure 7 and Table 1 show the signal efficiency and background rejection for varying thresholds on the output of the neural network (NN) or boosted decision tree (BDT).'' \\
% \cmidrule(l){2-5}
% & AI Model Adaptability &
% 100.0 &
% XGBoost: A Scalable Tree Boosting System, \textit{KDD}, 2016 &
% ``In this section, we evaluate the performance of XGBoost on a single machine using the exact greedy algorithm on Higgs-1M data, by comparing it against two other commonly used exact greedy tree boosting implementations.'' \\
% \midrule

% \multirow{2}{*}{\texttt{SUSY}} &
% AI Model Adaptability &
% 100.0 &
% \multirow{2}{=}{Searching for exotic particles in high-energy physics with deep learning, \textit{Nature Communications}, 2014} &
% ``In the case of the SUSY benchmark, the DNs again perform better than the shallow networks. The improvement is less dramatic, though statistically significant.'' \\
% \cmidrule(l){2-3}\cmidrule(l){5-5}
% & Task Generalizability &
% 89.0 & &
% ``This is a classification problem to distinguish between a signal process which produces supersymmetric particles and a background process which does not.'' \\
% \midrule

% \texttt{Laser\_Proton\_Accel.} &
% Task Generalizability &
% 100.0 &
% Stable laser-acceleration of high-flux proton beams with plasma collimation, \textit{Nature Communications}, 2025 &
% ``The simultaneous observation of several desirable beam properties at high repetition rate in this experiment is unprecedented in laser-driven proton acceleration.'' \\
% \midrule

% \texttt{Quantum\_Gas\_Light} &
% Task Generalizability &
% 93.0 &
% Dimensional crossover in a quantum gas of light, \textit{Nature Physics}, 2018 &
% ``Here, we observe the dimensional crossover from one to two dimensions in a harmonically trapped photon gas and study its properties.'' \\
% \midrule

% \multirow{2}{*}{\texttt{Quantum\_Metric\_Tensor}} &
% Accuracy &
% 100.0 &
% \multirow{2}{=}{Quantum Metric in Few-Layer Phosphorene, \textit{arXiv:2512.00914}, 2025} &
% ``In a recent study, Kim et al. have extracted the quantum metric components in black phosphorus by modeling it as an effective two-level system and measuring the corresponding pseudospins.'' \\
% \cmidrule(l){2-3}\cmidrule(l){5-5}
% & Task Generalizability &
% 100.0 & &
% ``While the QMT has been experimentally accessed in artificial platforms...and solids via techniques such as angle-resolved photoemission spectroscopy (ARPES), these measurements have so far been confined to electronic bands.'' \\


% \bottomrule
% \end{tabular}%
% }
% \end{table*}
